# Supplementary material for: A Competitive Deep Neural Network Approach for the ImageCLEFmed Caption 2020 Task
Source: arXiv:2007.14226 source file (2020-09-22)
Supplement: Supplementary file 1 [file appendix.tex]

\begin{table}[!ht]
\small
    \centering
    \begin{tabular}{|c | c |}
    \hline  %\toprule
    \rowcolor{cadetblue!55}
        Abbreviation       & Full form \\
    \hline \addlinespace[0.3em]    %\midrule
        DRAN    & DR Angiography      \\
    \rowcolor{gray!15}
        DRCO    & DR Combined modalities in One image     \\
        DRCT    & DR Computerized Tomography  \\
    \rowcolor{gray!15}
        DRMR    & DR Magenetic Resonance    \\
        DRPE    & DR Positron Emission Tomography   \\
    \rowcolor{gray!15}
        DRUS    & DR Ultrasound \\
        DRXR    & DR X-Ray, 2D Tomography \\
    \bottomrule
    \end{tabular}
    \vspace{1em}
    \caption{\label{table:roco-terminology} Terminology used in ``ROCO'' dataset.}
\end{table}
